# Supplementary material for: On the Learning and Learnability of Quasimetrics
Source: arXiv:2206.15478 source file (2022-10-04)
Supplement: Supplementary file 1 [file social_graph_berstan_full.tex]

%auto-ignore
%!TEX root = ../../../main.tex

\begin{adjustbox}{center}
\resizebox{
  1.25\linewidth
}{!}{%
\setlength{\tabcolsep}{4.5pt}
\renewcommand\normalsize{\small}%
\normalsize
\makeatletter
\newcommand{\dispone}[2]{
   \ifthenelse{\equal{#1}{nan}}
    {\texttt{NaN}}
    {%
    \ifthenelse{\equal{#1}{inf}}
        {$\infty$}
        {%
        \fpcmpTF{abs(#1)<=10000}{%
            \num[round-precision=#2,round-mode=places,scientific-notation=fixed,group-minimum-digits=100,fixed-exponent=0,mode=text,detect-weight=true,detect-family=true]{#1}%
        }{%
            \num[round-precision=#2,round-mode=places,scientific-notation=true,group-minimum-digits=100,mode=text,detect-weight=true,detect-family=true]{#1}%
        }
        }%
    }%
}
\makeatother
\newcommand{\disp}[4]{\dispone{#1}{#2}$~\pm$\dispone{#3}{#4}}
\begin{tabular}[b]{cllccc}
    \toprule
    \multirow{3}{*}{Method Family}
    &
    \multicolumn{2}{c}{\multirow{3}{*}{Formulation}}
    % &
    &  \multirow{3}{*}{\vspace{0pt}\shortstack{MSE \wrt\\[0.6ex]$\gamma$-discounted\\[0.1ex]distances $(\times 10^{-3})$ $\boldsymbol\downarrow$}}
    &  \multirow{3}{*}{\vspace{1pt}\shortstack{L1 Error\\[0.6ex]when true\\[0.8ex]$d < \infty$  $\boldsymbol\downarrow$}}
    &  \multirow{3}{*}{\vspace{2pt}\shortstack{Prediction $\hat{d}$\\[0.6ex]when true\\[0.8ex]$d = \infty$  $\boldsymbol\uparrow$}} \\
    &
    &
    &
    &
    &   \\
    &
    &
    &
    &
    &   \\[-0.4ex]
    \midrule
    \midrule

    \multirow{2}{*}{PQEs} &
    PQE-LH
    &
    & \disp{3.0426766257733107}{4}{0.1527027714084911}{4}
    & \disp{1.626337456703186}{4}{0.05502454904769019}{4}
    & \disp{69.94242248535156}{4}{0.4930275855506096}{4}
    \\

    &
    PQE-GG
    &
    & \disp{3.908537095412612}{4}{0.12580057445957663}{4}
    & \disp{1.895107340812683}{4}{0.03359626265223329}{4}
    & \disp{101.82395477294922}{4}{10.39697492748484}{4}
    \\
    \hline

    \multirow{5}{*}{\vspace{0pt}\shortstack{\Uncon Nets\\\\(without Triangle Inequality\\Regularizer)}}
    & Output distance
    & $\hat{d}(x, y) \trieq f(x, y)$
    & \disp{3.0862420331686735}{4}{0.03916676919711341}{4}
    & \disp{2.1151447772979735}{4}{0.024078517111510263}{4}
    & \disp{59.5242919921875}{4}{0.37004197274349077}{4}
    \\
    & Output distance via $\exp(\cdot)$
    & $\hat{d}(x, y) \trieq \exp(f(x, y))$
    & \disp{3.354074840899557}{4}{0.17594723668687823}{4}
    & \disp{1.0089520530149328e+23}{4}{2.0179041060298656e+23}{4}
    & \disp{535827.3560791016}{4}{1058247.3726819062}{4}
    \\
    & Output distance via squaring $a \rightarrow a^2$
    & $\hat{d}(x, y) \trieq (f(x, y))^2$
    & \disp{4.566348809748888}{4}{0.2293880375948404}{4}
    & \disp{3.3458715438842774}{4}{0.24944923172568575}{4}
    & \disp{68.26129150390625}{4}{11.606111334456381}{4}
    \\
    & Output $\gamma$-discounted distance
    & $\gamma^{\hat{d}(x, y)} \trieq f(x, y)$
    & \disp{nan}{4}{nan}{4}
    & \disp{nan}{4}{nan}{4}
    & \disp{nan}{4}{nan}{4}
    \\
    & Output $\gamma$-discounted distance via sigmoid $\sigma(\cdot)$
    & $\gamma^{\hat{d}(x, y)} \trieq \sigma(f(x, y))$
    & \disp{3.1822795048356056}{4}{0.1133211265922544}{4}
    & \disp{inf}{4}{nan}{4}
    & \disp{65.86301727294922}{4}{0.42867235969927625}{4}
    \\
    \hline

    \multirow{5}{*}{\vspace{0pt}\shortstack{\Uncon Nets\\\\(Triangle Inequality\\Regularizer Weight $=0.3$)}}
    & Output distance
    & $\hat{d}(x, y) \trieq f(x, y)$
    & \disp{2.8128044679760933}{4}{0.06251623447057535}{4}
    & \disp{2.210947322845459}{4}{0.034070232889604174}{4}
    & \disp{61.37094268798828}{4}{0.3935568080866707}{4}
    \\
    & Output distance via $\exp(\cdot)$
    & $\hat{d}(x, y) \trieq \exp(f(x, y))$
    & \disp{2.9343554750084877}{4}{0.045537305699257236}{4}
    & \disp{inf}{4}{nan}{4}
    & \disp{inf}{4}{nan}{4}
    \\
    & Output distance via squaring $a \rightarrow a^2$
    & $\hat{d}(x, y) \trieq (f(x, y))^2$
    & \disp{4.994736518710852}{4}{0.419816860877629}{4}
    & \disp{16.544499397277832}{4}{29.31746780544482}{4}
    & \disp{58.92046203613281}{4}{6.421621636225229}{4}
    \\
    & Output $\gamma$-discounted distance
    & $\gamma^{\hat{d}(x, y)} \trieq f(x, y)$
    & \disp{nan}{4}{nan}{4}
    & \disp{nan}{4}{nan}{4}
    & \disp{nan}{4}{nan}{4}
    \\
    & Output $\gamma$-discounted distance via sigmoid $\sigma(\cdot)$
    & $\gamma^{\hat{d}(x, y)} \trieq \sigma(f(x, y))$
    & \disp{2.917815512046218}{4}{0.13513306914275294}{4}
    & \disp{inf}{4}{nan}{4}
    & \disp{inf}{4}{nan}{4}
    \\
    \hline

    \multirow{5}{*}{\vspace{0pt}\shortstack{\Uncon Nets\\\\(Triangle Inequality\\Regularizer Weight $=1$)}}
    & Output distance
    & $\hat{d}(x, y) \trieq f(x, y)$
    & \disp{3.048108145594597}{4}{0.12717510500606136}{4}
    & \disp{2.372862195968628}{4}{0.1377995383563425}{4}
    & \disp{60.40402450561523}{4}{0.1889967397389779}{4}
    \\
    & Output distance via $\exp(\cdot)$
    & $\hat{d}(x, y) \trieq \exp(f(x, y))$
    & \disp{3.016129310708493}{4}{0.07183977055958074}{4}
    & \disp{inf}{4}{nan}{4}
    & \disp{3.128940583453215e+16}{4}{6.257881166904982e+16}{4}
    \\
    & Output distance via squaring $a \rightarrow a^2$
    & $\hat{d}(x, y) \trieq (f(x, y))^2$
    & \disp{4.492051433771849}{4}{0.35341492946085384}{4}
    & \disp{3.6929863929748534}{4}{0.48959212332367835}{4}
    & \disp{90.62057189941406}{4}{66.57044725907389}{4}
    \\
    & Output $\gamma$-discounted distance
    & $\gamma^{\hat{d}(x, y)} \trieq f(x, y)$
    & \disp{4.404620034620166}{4}{0.5167470337961341}{4}
    & \disp{2.7873454093933105}{4}{0.07704389698563949}{4}
    & \disp{31.319485982259113}{4}{0.992932202888254}{4}
    \\
    & Output $\gamma$-discounted distance via sigmoid $\sigma(\cdot)$
    & $\gamma^{\hat{d}(x, y)} \trieq \sigma(f(x, y))$
    & \disp{2.931429725140333}{4}{0.10217073276646424}{4}
    & \disp{2.2633790969848633}{4}{0.11472897339265811}{4}
    & \disp{inf}{4}{nan}{4}
    \\
    \hline

    \multirow{5}{*}{\vspace{0pt}\shortstack{\Uncon Nets\\\\(Triangle Inequality\\Regularizer Weight $=3$)}}
    & Output distance
    & $\hat{d}(x, y) \trieq f(x, y)$
    & \disp{5.295455362647772}{4}{0.5279059600868634}{4}
    & \disp{3.8059605598449706}{4}{0.2908288386558469}{4}
    & \disp{58.119309997558595}{4}{0.4383464891543171}{4}
    \\
    & Output distance via $\exp(\cdot)$
    & $\hat{d}(x, y) \trieq \exp(f(x, y))$
    & \disp{3.5712829558178782}{4}{0.20015522733362273}{4}
    & \disp{212.5421069264412}{4}{416.92559900081045}{4}
    & \disp{inf}{4}{nan}{4}
    \\
    & Output distance via squaring $a \rightarrow a^2$
    & $\hat{d}(x, y) \trieq (f(x, y))^2$
    & \disp{4.374542972072959}{4}{0.3709305725242967}{4}
    & \disp{2.949071502685547}{4}{0.22277117585697476}{4}
    & \disp{53.11185150146484}{4}{5.545150300899283}{4}
    \\
    & Output $\gamma$-discounted distance
    & $\gamma^{\hat{d}(x, y)} \trieq f(x, y)$
    & \disp{7.341564865782857}{4}{0.6486245227867216}{4}
    & \disp{3.5231974124908447}{4}{0.13522890297957127}{4}
    & \disp{26.920034408569336}{4}{0.46972224338166885}{4}
    \\
    & Output $\gamma$-discounted distance via sigmoid $\sigma(\cdot)$
    & $\gamma^{\hat{d}(x, y)} \trieq \sigma(f(x, y))$
    & \disp{3.581829881295562}{4}{0.35652750938302397}{4}
    & \disp{inf}{4}{nan}{4}
    & \disp{65.77092895507812}{4}{0.8646475408973068}{4}
    \\
    \hline

    \multirow{5}{*}{\vspace{0pt}\shortstack{Asym.~Dot Products\\\\(without Triangle Inequality\\Regularizer)}}
    & Output distance
    & $\hat{d}(x, y) \trieq f(x)\T g(y)$
    & \disp{3.1621926497550336e+19}{4}{nan}{4}
    & \disp{23.426950454711914}{4}{nan}{4}
    & \disp{0.1529184728860855}{4}{nan}{4}
    \\
    & Output distance via $\exp(\cdot)$
    & $\hat{d}(x, y) \trieq \exp(f(x)\T g(y))$
    & \disp{nan}{4}{nan}{4}
    & \disp{nan}{4}{nan}{4}
    & \disp{nan}{4}{nan}{4}
    \\
    & Output distance via squaring $a \rightarrow a^2$
    & $\hat{d}(x, y) \trieq (f(x)\T g(y))^2$
    & \disp{48.105619102716446}{4}{0.005621992204445349}{4}
    & \disp{251953764761.6}{4}{217507391823.59286}{4}
    & \disp{267943034880.0}{4}{253982361506.07498}{4}
    \\
    & Output $\gamma$-discounted distance
    & $\gamma^{\hat{d}(x, y)} \trieq f(x)\T g(y)$
    & \disp{nan}{4}{nan}{4}
    & \disp{nan}{4}{nan}{4}
    & \disp{nan}{4}{nan}{4}
    \\
    & Output $\gamma$-discounted distance via sigmoid $\sigma(\cdot)$
    & $\gamma^{\hat{d}(x, y)} \trieq \sigma(f(x)\T g(y))$
    & \disp{48.1072798371315}{4}{0.011200521150776063}{4}
    & \disp{inf}{4}{nan}{4}
    & \disp{inf}{4}{nan}{4}
    \\
    \hline

    \multirow{5}{*}{\vspace{0pt}\shortstack{Asym.~Dot Products\\\\(Triangle Inequality\\Regularizer Weight $=0.3$)}}
    & Output distance
    & $\hat{d}(x, y) \trieq f(x)\T g(y)$
    & \disp{nan}{4}{nan}{4}
    & \disp{nan}{4}{nan}{4}
    & \disp{nan}{4}{nan}{4}
    \\
    & Output distance via $\exp(\cdot)$
    & $\hat{d}(x, y) \trieq \exp(f(x)\T g(y))$
    & \disp{nan}{4}{nan}{4}
    & \disp{nan}{4}{nan}{4}
    & \disp{nan}{4}{nan}{4}
    \\
    & Output distance via squaring $a \rightarrow a^2$
    & $\hat{d}(x, y) \trieq (f(x)\T g(y))^2$
    & \disp{48.104140907526016}{4}{0.003455732369383177}{4}
    & \disp{194977018675.2}{4}{79641434469.06987}{4}
    & \disp{160491628134.4}{4}{37098616579.97885}{4}
    \\
    & Output $\gamma$-discounted distance
    & $\gamma^{\hat{d}(x, y)} \trieq f(x)\T g(y)$
    & \disp{nan}{4}{nan}{4}
    & \disp{nan}{4}{nan}{4}
    & \disp{nan}{4}{nan}{4}
    \\
    & Output $\gamma$-discounted distance via sigmoid $\sigma(\cdot)$
    & $\gamma^{\hat{d}(x, y)} \trieq \sigma(f(x)\T g(y))$
    & \disp{48.110271245241165}{4}{0.010955044669081407}{4}
    & \disp{inf}{4}{nan}{4}
    & \disp{inf}{4}{nan}{4}
    \\
    \hline

    \multirow{5}{*}{\vspace{0pt}\shortstack{Asym.~Dot Products\\\\(Triangle Inequality\\Regularizer Weight $=1$)}}
    & Output distance
    & $\hat{d}(x, y) \trieq f(x)\T g(y)$
    & \disp{nan}{4}{nan}{4}
    & \disp{nan}{4}{nan}{4}
    & \disp{nan}{4}{nan}{4}
    \\
    & Output distance via $\exp(\cdot)$
    & $\hat{d}(x, y) \trieq \exp(f(x)\T g(y))$
    & \disp{nan}{4}{nan}{4}
    & \disp{nan}{4}{nan}{4}
    & \disp{nan}{4}{nan}{4}
    \\
    & Output distance via squaring $a \rightarrow a^2$
    & $\hat{d}(x, y) \trieq (f(x)\T g(y))^2$
    & \disp{48.102133721113205}{4}{0.0002099325861824455}{4}
    & \disp{229862739148.8}{4}{91969693443.19614}{4}
    & \disp{250022690816.0}{4}{144640363009.09177}{4}
    \\
    & Output $\gamma$-discounted distance
    & $\gamma^{\hat{d}(x, y)} \trieq f(x)\T g(y)$
    & \disp{nan}{4}{nan}{4}
    & \disp{nan}{4}{nan}{4}
    & \disp{nan}{4}{nan}{4}
    \\
    & Output $\gamma$-discounted distance via sigmoid $\sigma(\cdot)$
    & $\gamma^{\hat{d}(x, y)} \trieq \sigma(f(x)\T g(y))$
    & \disp{58.489375561475754}{4}{23.222417793063986}{4}
    & \disp{inf}{4}{nan}{4}
    & \disp{inf}{4}{nan}{4}
    \\
    \hline

    \multirow{5}{*}{\vspace{0pt}\shortstack{Asym.~Dot Products\\\\(Triangle Inequality\\Regularizer Weight $=3$)}}
    & Output distance
    & $\hat{d}(x, y) \trieq f(x)\T g(y)$
    & \disp{nan}{4}{nan}{4}
    & \disp{nan}{4}{nan}{4}
    & \disp{nan}{4}{nan}{4}
    \\
    & Output distance via $\exp(\cdot)$
    & $\hat{d}(x, y) \trieq \exp(f(x)\T g(y))$
    & \disp{nan}{4}{nan}{4}
    & \disp{nan}{4}{nan}{4}
    & \disp{nan}{4}{nan}{4}
    \\
    & Output distance via squaring $a \rightarrow a^2$
    & $\hat{d}(x, y) \trieq (f(x)\T g(y))^2$
    & \disp{48.1030635535717}{4}{0.001969282674127401}{4}
    & \disp{235218866995.2}{4}{264292093502.76407}{4}
    & \disp{170245775360.0}{4}{106996783774.62538}{4}
    \\
    & Output $\gamma$-discounted distance
    & $\gamma^{\hat{d}(x, y)} \trieq f(x)\T g(y)$
    & \disp{nan}{4}{nan}{4}
    & \disp{nan}{4}{nan}{4}
    & \disp{nan}{4}{nan}{4}
    \\
    & Output $\gamma$-discounted distance via sigmoid $\sigma(\cdot)$
    & $\gamma^{\hat{d}(x, y)} \trieq \sigma(f(x)\T g(y))$
    & \disp{48.30335974693298}{4}{0.4485206653057057}{4}
    & \disp{inf}{4}{nan}{4}
    & \disp{inf}{4}{nan}{4}
    \\
    \hline

    \multirow{4}{*}{Metric Embeddings}
    & Euclidean space
    & $\hat{d}(x, y)\trieq \norm{f(x) - f(y)}_2$
    & \disp{17.595218867063522}{4}{0.26668822519713126}{4}
    & \disp{7.539879989624024}{4}{0.07420489860935446}{4}
    & \disp{53.85003433227539}{4}{3.843024787898114}{4}
    \\
    & $\ell_1$ space
    & $\hat{d}(x, y)\trieq \norm{f(x) - f(y)}_1$
    & \disp{18.05211342871189}{4}{0.35458909249787296}{4}
    & \disp{7.115421772003174}{4}{0.183545049465368}{4}
    & \disp{66.25067901611328}{4}{3.3308028502344964}{4}
    \\
    & Spherical distance space w/ learnable scale $\alpha$
    & $\hat{d}(x, y)\trieq \alpha \cdot \arccos(\frac{f(x)\T f(y)}{\norm{f(x)}_2 \norm{f(y)}_2})$
    & \disp{19.299031421542168}{4}{0.2032374641976178}{4}
    & \disp{6.954515171051026}{4}{0.08871404006349713}{4}
    & \disp{32.14578132629394}{4}{0.45622836495469177}{4}
    \\
    & Mixing above three spaces w/ learnable weights
    &
    & \disp{17.83115714788437}{4}{0.30987170679673604}{4}
    & \disp{7.349317741394043}{4}{0.10858450937050752}{4}
    & \disp{51.7480972290039}{4}{3.6248379063359786}{4}
    \\
    \hline

    \multirow{2}{*}{DeepNorms} &
    $3$-layer $128$-width
    &
    & \disp{7.086162082850933}{4}{0.3169639087122429}{4}
    & \disp{2.4497997760772705}{4}{0.061715361982906204}{4}
    & \disp{111.22088928222657}{4}{2.504455572940638}{4}
    \\

    &
    $3$-layer $512$-width
    &
    & \disp{5.071479082107544}{4}{0.13476357031416314}{4}
    & \disp{2.0852701663970947}{4}{0.0632648640792226}{4}
    & \disp{120.04515838623047}{4}{4.352518794402874}{4}
    \\
    \hline

    \multirow{3}{*}{WideNorms} &
    $32$-component (each of size $32$)
    &
    & \disp{3.532807668671012}{4}{0.21201393857838322}{4}
    & \disp{1.769381594657898}{4}{0.02132951306760224}{4}
    & \disp{124.65802764892578}{4}{2.8677826229958154}{4}
    \\

    &
    $48$-component (each of size $32$)
    &
    & \disp{3.684179112315178}{4}{0.2385308584382033}{4}
    & \disp{1.8081010103225708}{4}{0.06796887705493833}{4}
    & \disp{122.68327941894532}{4}{5.50260682750137}{4}
    \\

    &
    $128$-component (each of size $32$)
    &
    & \disp{3.8124782033264637}{4}{0.2331290555050261}{4}
    & \disp{1.8096019983291627}{4}{0.07645060876884974}{4}
    & \disp{128.54269409179688}{4}{5.141237660831908}{4}
    \\
    \bottomrule
\end{tabular}%
}
\end{adjustbox}
