# Supplementary material for: On the Learning and Learnability of Quasimetrics
Source: arXiv:2206.15478 source file (2022-10-04)
Supplement: Supplementary file 2 [file social_graph_youtube_full.tex]

%auto-ignore
%!TEX root = ../../../main.tex
\begin{adjustbox}{center}
\resizebox{
  1.25\linewidth
}{!}{%
\setlength{\tabcolsep}{4.5pt}
\renewcommand\normalsize{\small}%
\normalsize
\makeatletter
\newcommand{\dispone}[2]{
   \ifthenelse{\equal{#1}{nan}}
    {\texttt{NaN}}
    {%
    \ifthenelse{\equal{#1}{inf}}
        {$\infty$}
        {%
        \fpcmpTF{abs(#1)<=10000}{%
            \num[round-precision=#2,round-mode=places,scientific-notation=fixed,group-minimum-digits=100,fixed-exponent=0,mode=text,detect-weight=true,detect-family=true]{#1}%
        }{%
            \num[round-precision=#2,round-mode=places,scientific-notation=true,group-minimum-digits=100,mode=text,detect-weight=true,detect-family=true]{#1}%
        }
        }%
    }%
}
\makeatother
\newcommand{\disp}[4]{\dispone{#1}{#2}$~\pm$\dispone{#3}{#4}}
\begin{tabular}[b]{cllccc}
    \toprule
    \multirow{3}{*}{Method Family}
    &
    \multicolumn{2}{c}{\multirow{3}{*}{Formulation}}
    % &
    &  \multirow{3}{*}{\vspace{0pt}\shortstack{MSE \wrt\\[0.6ex]$\gamma$-discounted\\[0.1ex]distances $(\times 10^{-3})$ $\boldsymbol\downarrow$}}
    &  \multirow{3}{*}{\vspace{1pt}\shortstack{L1 Error\\[0.6ex]when true\\[0.8ex]$d < \infty$  $\boldsymbol\downarrow$}}
    &  \multirow{3}{*}{\vspace{2pt}\shortstack{Prediction $\hat{d}$\\[0.6ex]when true\\[0.8ex]$d = \infty$  $\boldsymbol\uparrow$}} \\
    &
    &
    &
    &
    &   \\
    &
    &
    &
    &
    &   \\[-0.4ex]
    \midrule
    \midrule

    \multirow{2}{*}{PQEs} &
    PQE-LH
    &
    & \disp{2.439998695626855}{4}{0.06945692541884159}{4}
    & \disp{0.6479844927787781}{4}{0.011867603420750269}{4}
    & \disp{nan}{4}{nan}{4}
    \\

    &
    PQE-GG
    &
    & \disp{2.589528728276491}{4}{0.03175171226752573}{4}
    & \disp{0.6697321534156799}{4}{0.004184238661891272}{4}
    & \disp{nan}{4}{nan}{4}
    \\
    \hline

    \multirow{5}{*}{\vspace{0pt}\shortstack{\Uncon Nets\\\\(without Triangle Inequality\\Regularizer)}}
    & Output distance
    & $\hat{d}(x, y) \trieq f(x, y)$
    & \disp{1.488293963484466}{4}{0.01677136161047181}{4}
    & \disp{0.5083753824234009}{4}{0.0029362765879703805}{4}
    & \disp{nan}{4}{nan}{4}
    \\
    & Output distance via $\exp(\cdot)$
    & $\hat{d}(x, y) \trieq \exp(f(x, y))$
    & \disp{1.5222502406686544}{4}{0.016039933907932704}{4}
    & \disp{0.49098752737045287}{4}{0.015081251521296858}{4}
    & \disp{nan}{4}{nan}{4}
    \\
    & Output distance via squaring $a \rightarrow a^2$
    & $\hat{d}(x, y) \trieq (f(x, y))^2$
    & \disp{2.295490959659219}{4}{1.16740741992376}{4}
    & \disp{0.618457418680191}{4}{0.14087950627529422}{4}
    & \disp{nan}{4}{nan}{4}
    \\
    & Output $\gamma$-discounted distance
    & $\gamma^{\hat{d}(x, y)} \trieq f(x, y)$
    & \disp{1.5068939188495278}{4}{0.022845189463368186}{4}
    & \disp{0.497537225484848}{4}{0.021094923050397948}{4}
    & \disp{nan}{4}{nan}{4}
    \\
    & Output $\gamma$-discounted distance via sigmoid $\sigma(\cdot)$
    & $\gamma^{\hat{d}(x, y)} \trieq \sigma(f(x, y))$
    & \disp{1.4802108751609921}{4}{0.019671309251206963}{4}
    & \disp{0.5081566572189331}{4}{0.0035935111084154673}{4}
    & \disp{nan}{4}{nan}{4}
    \\
    \hline

    \multirow{5}{*}{\vspace{0pt}\shortstack{\Uncon Nets\\\\(Triangle Inequality\\Regularizer Weight $=0.3$)}}
    & Output distance
    & $\hat{d}(x, y) \trieq f(x, y)$
    & \disp{1.5009395545348525}{4}{0.020845460776718436}{4}
    & \disp{0.5106761693954468}{4}{0.0032323978476644544}{4}
    & \disp{nan}{4}{nan}{4}
    \\
    & Output distance via $\exp(\cdot)$
    & $\hat{d}(x, y) \trieq \exp(f(x, y))$
    & \disp{1.5205684583634138}{4}{0.04443725527845903}{4}
    & \disp{0.49346142411231997}{4}{0.009798898715540096}{4}
    & \disp{nan}{4}{nan}{4}
    \\
    & Output distance via squaring $a \rightarrow a^2$
    & $\hat{d}(x, y) \trieq (f(x, y))^2$
    & \disp{1.739829103462398}{4}{0.38959710509523915}{4}
    & \disp{0.548811399936676}{4}{0.06000373304786795}{4}
    & \disp{nan}{4}{nan}{4}
    \\
    & Output $\gamma$-discounted distance
    & $\gamma^{\hat{d}(x, y)} \trieq f(x, y)$
    & \disp{1.5005233697593212}{4}{0.014750703440312185}{4}
    & \disp{0.4985992729663849}{4}{0.012073256249042971}{4}
    & \disp{nan}{4}{nan}{4}
    \\
    & Output $\gamma$-discounted distance via sigmoid $\sigma(\cdot)$
    & $\gamma^{\hat{d}(x, y)} \trieq \sigma(f(x, y))$
    & \disp{1.485149934887886}{4}{0.016839516514275437}{4}
    & \disp{0.5089208602905273}{4}{0.0025600761243137404}{4}
    & \disp{nan}{4}{nan}{4}
    \\
    \hline

    \multirow{5}{*}{\vspace{0pt}\shortstack{\Uncon Nets\\\\(Triangle Inequality\\Regularizer Weight $=1$)}}
    & Output distance
    & $\hat{d}(x, y) \trieq f(x, y)$
    & \disp{1.4999430859461427}{4}{0.024339616308195044}{4}
    & \disp{0.5106872677803039}{4}{0.004638251142549701}{4}
    & \disp{nan}{4}{nan}{4}
    \\
    & Output distance via $\exp(\cdot)$
    & $\hat{d}(x, y) \trieq \exp(f(x, y))$
    & \disp{1.5223789494484663}{4}{0.03761170443505153}{4}
    & \disp{0.4948307156562805}{4}{0.016915634902460123}{4}
    & \disp{nan}{4}{nan}{4}
    \\
    & Output distance via squaring $a \rightarrow a^2$
    & $\hat{d}(x, y) \trieq (f(x, y))^2$
    & \disp{1.8875153036788106}{4}{0.5077693034466935}{4}
    & \disp{0.5692490935325623}{4}{0.06826322357598065}{4}
    & \disp{nan}{4}{nan}{4}
    \\
    & Output $\gamma$-discounted distance
    & $\gamma^{\hat{d}(x, y)} \trieq f(x, y)$
    & \disp{1.4768982073292136}{4}{0.017596401642142774}{4}
    & \disp{0.491934472322464}{4}{0.012784444321095512}{4}
    & \disp{nan}{4}{nan}{4}
    \\
    & Output $\gamma$-discounted distance via sigmoid $\sigma(\cdot)$
    & $\gamma^{\hat{d}(x, y)} \trieq \sigma(f(x, y))$
    & \disp{1.4846331905573606}{4}{0.011538219754186051}{4}
    & \disp{0.5088278174400329}{4}{0.0020679558134244396}{4}
    & \disp{nan}{4}{nan}{4}
    \\
    \hline

    \multirow{5}{*}{\vspace{0pt}\shortstack{\Uncon Nets\\\\(Triangle Inequality\\Regularizer Weight $=3$)}}
    & Output distance
    & $\hat{d}(x, y) \trieq f(x, y)$
    & \disp{1.4938974287360907}{4}{0.010999750653482288}{4}
    & \disp{0.5099177122116089}{4}{0.0018209613602228395}{4}
    & \disp{nan}{4}{nan}{4}
    \\
    & Output distance via $\exp(\cdot)$
    & $\hat{d}(x, y) \trieq \exp(f(x, y))$
    & \disp{1.515410584397614}{4}{0.038863817894616286}{4}
    & \disp{0.4871287286281586}{4}{0.017447881084738003}{4}
    & \disp{nan}{4}{nan}{4}
    \\
    & Output distance via squaring $a \rightarrow a^2$
    & $\hat{d}(x, y) \trieq (f(x, y))^2$
    & \disp{2.474687877111137}{4}{1.085025113012615}{4}
    & \disp{0.6504552602767945}{4}{0.13569607846946738}{4}
    & \disp{nan}{4}{nan}{4}
    \\
    & Output $\gamma$-discounted distance
    & $\gamma^{\hat{d}(x, y)} \trieq f(x, y)$
    & \disp{1.491524837911129}{4}{0.012667630288700589}{4}
    & \disp{0.49833652973175047}{4}{0.016002778281961012}{4}
    & \disp{nan}{4}{nan}{4}
    \\
    & Output $\gamma$-discounted distance via sigmoid $\sigma(\cdot)$
    & $\gamma^{\hat{d}(x, y)} \trieq \sigma(f(x, y))$
    & \disp{1.4828914310783148}{4}{0.01531842337566277}{4}
    & \disp{0.5084498047828674}{4}{0.0028775660231187498}{4}
    & \disp{nan}{4}{nan}{4}
    \\
    \hline

    \multirow{5}{*}{\vspace{0pt}\shortstack{Asym.~Dot Products\\\\(without Triangle Inequality\\Regularizer)}}
    & Output distance
    & $\hat{d}(x, y) \trieq f(x)\T g(y)$
    & \disp{2633.7907314300537}{4}{nan}{4}
    & \disp{11.387887954711914}{4}{nan}{4}
    & \disp{nan}{4}{nan}{4}
    \\
    & Output distance via $\exp(\cdot)$
    & $\hat{d}(x, y) \trieq \exp(f(x)\T g(y))$
    & \disp{nan}{4}{nan}{4}
    & \disp{nan}{4}{nan}{4}
    & \disp{nan}{4}{nan}{4}
    \\
    & Output distance via squaring $a \rightarrow a^2$
    & $\hat{d}(x, y) \trieq (f(x)\T g(y))^2$
    & \disp{339.1550064086914}{4}{0.002207042570308556}{4}
    & \disp{789481383526.4}{4}{740100205124.2113}{4}
    & \disp{nan}{4}{nan}{4}
    \\
    & Output $\gamma$-discounted distance
    & $\gamma^{\hat{d}(x, y)} \trieq f(x)\T g(y)$
    & \disp{2.691951231099665}{4}{1.2655193571413337}{4}
    & \disp{0.7061967651049296}{4}{0.21562210169241638}{4}
    & \disp{nan}{4}{nan}{4}
    \\
    & Output $\gamma$-discounted distance via sigmoid $\sigma(\cdot)$
    & $\gamma^{\hat{d}(x, y)} \trieq \sigma(f(x)\T g(y))$
    & \disp{182.2068214416504}{4}{1.238189534765879}{4}
    & \disp{inf}{4}{nan}{4}
    & \disp{nan}{4}{nan}{4}
    \\
    \hline

    \multirow{5}{*}{\vspace{0pt}\shortstack{Asym.~Dot Products\\\\(Triangle Inequality\\Regularizer Weight $=0.3$)}}
    & Output distance
    & $\hat{d}(x, y) \trieq f(x)\T g(y)$
    & \disp{997481.5673828125}{4}{nan}{4}
    & \disp{8.186738014221191}{4}{nan}{4}
    & \disp{nan}{4}{nan}{4}
    \\
    & Output distance via $\exp(\cdot)$
    & $\hat{d}(x, y) \trieq \exp(f(x)\T g(y))$
    & \disp{nan}{4}{nan}{4}
    & \disp{nan}{4}{nan}{4}
    & \disp{nan}{4}{nan}{4}
    \\
    & Output distance via squaring $a \rightarrow a^2$
    & $\hat{d}(x, y) \trieq (f(x)\T g(y))^2$
    & \disp{339.1560137271881}{4}{0.0010301434734335357}{4}
    & \disp{686576481075.2}{4}{349850546520.6418}{4}
    & \disp{nan}{4}{nan}{4}
    \\
    & Output $\gamma$-discounted distance
    & $\gamma^{\hat{d}(x, y)} \trieq f(x)\T g(y)$
    & \disp{nan}{4}{nan}{4}
    & \disp{nan}{4}{nan}{4}
    & \disp{nan}{4}{nan}{4}
    \\
    & Output $\gamma$-discounted distance via sigmoid $\sigma(\cdot)$
    & $\gamma^{\hat{d}(x, y)} \trieq \sigma(f(x)\T g(y))$
    & \disp{183.33366513252258}{4}{1.038441529612902}{4}
    & \disp{inf}{4}{nan}{4}
    & \disp{nan}{4}{nan}{4}
    \\
    \hline

    \multirow{5}{*}{\vspace{0pt}\shortstack{Asym.~Dot Products\\\\(Triangle Inequality\\Regularizer Weight $=1$)}}
    & Output distance
    & $\hat{d}(x, y) \trieq f(x)\T g(y)$
    & \disp{nan}{4}{nan}{4}
    & \disp{nan}{4}{nan}{4}
    & \disp{nan}{4}{nan}{4}
    \\
    & Output distance via $\exp(\cdot)$
    & $\hat{d}(x, y) \trieq \exp(f(x)\T g(y))$
    & \disp{nan}{4}{nan}{4}
    & \disp{nan}{4}{nan}{4}
    & \disp{nan}{4}{nan}{4}
    \\
    & Output distance via squaring $a \rightarrow a^2$
    & $\hat{d}(x, y) \trieq (f(x)\T g(y))^2$
    & \disp{339.1551733016968}{4}{0.0021355396815898368}{4}
    & \disp{745881803161.6}{4}{372773897079.66754}{4}
    & \disp{nan}{4}{nan}{4}
    \\
    & Output $\gamma$-discounted distance
    & $\gamma^{\hat{d}(x, y)} \trieq f(x)\T g(y)$
    & \disp{nan}{4}{nan}{4}
    & \disp{nan}{4}{nan}{4}
    & \disp{nan}{4}{nan}{4}
    \\
    & Output $\gamma$-discounted distance via sigmoid $\sigma(\cdot)$
    & $\gamma^{\hat{d}(x, y)} \trieq \sigma(f(x)\T g(y))$
    & \disp{191.092848777771}{4}{9.713728867294533}{4}
    & \disp{inf}{4}{nan}{4}
    & \disp{nan}{4}{nan}{4}
    \\
    \hline

    \multirow{5}{*}{\vspace{0pt}\shortstack{Asym.~Dot Products\\\\(Triangle Inequality\\Regularizer Weight $=3$)}}
    & Output distance
    & $\hat{d}(x, y) \trieq f(x)\T g(y)$
    & \disp{nan}{4}{nan}{4}
    & \disp{nan}{4}{nan}{4}
    & \disp{nan}{4}{nan}{4}
    \\
    & Output distance via $\exp(\cdot)$
    & $\hat{d}(x, y) \trieq \exp(f(x)\T g(y))$
    & \disp{nan}{4}{nan}{4}
    & \disp{nan}{4}{nan}{4}
    & \disp{nan}{4}{nan}{4}
    \\
    & Output distance via squaring $a \rightarrow a^2$
    & $\hat{d}(x, y) \trieq (f(x)\T g(y))^2$
    & \disp{339.1555905342102}{4}{0.0020078893103643667}{4}
    & \disp{902832573644.8}{4}{602031629255.6624}{4}
    & \disp{nan}{4}{nan}{4}
    \\
    & Output $\gamma$-discounted distance
    & $\gamma^{\hat{d}(x, y)} \trieq f(x)\T g(y)$
    & \disp{nan}{4}{nan}{4}
    & \disp{nan}{4}{nan}{4}
    & \disp{nan}{4}{nan}{4}
    \\
    & Output $\gamma$-discounted distance via sigmoid $\sigma(\cdot)$
    & $\gamma^{\hat{d}(x, y)} \trieq \sigma(f(x)\T g(y))$
    & \disp{228.0300408601761}{4}{37.06323693023475}{4}
    & \disp{inf}{4}{nan}{4}
    & \disp{nan}{4}{nan}{4}
    \\
    \hline

    \multirow{4}{*}{Metric Embeddings}
    & Euclidean space
    & $\hat{d}(x, y)\trieq \norm{f(x) - f(y)}_2$
    & \disp{1.313072140328586}{4}{0.06709181528252355}{4}
    & \disp{0.48333577513694764}{4}{0.012823285300940044}{4}
    & \disp{nan}{4}{nan}{4}
    \\
    & $\ell_1$ space
    & $\hat{d}(x, y)\trieq \norm{f(x) - f(y)}_1$
    & \disp{3.599314112216234}{4}{1.5985805414335168}{4}
    & \disp{0.7786912083625793}{4}{0.18424971703893092}{4}
    & \disp{nan}{4}{nan}{4}
    \\
    & Spherical distance space w/ learnable scale $\alpha$
    & $\hat{d}(x, y)\trieq \alpha \cdot \arccos(\frac{f(x)\T f(y)}{\norm{f(x)}_2 \norm{f(y)}_2})$
    & \disp{6.773118861019611}{4}{0.1914659340240271}{4}
    & \disp{1.082905650138855}{4}{0.01770966133258167}{4}
    & \disp{nan}{4}{nan}{4}
    \\
    & Mixing above three spaces w/ learnable weights
    &
    & \disp{2.101387223228812}{4}{0.06854888198258723}{4}
    & \disp{0.592292058467865}{4}{0.010935059255615907}{4}
    & \disp{nan}{4}{nan}{4}
    \\
    \hline

    \multirow{2}{*}{DeepNorms} &
    $3$-layer $128$-width
    &
    & \disp{8.019166067242622}{4}{0.24760360872265116}{4}
    & \disp{1.1833733081817628}{4}{0.021319486782568647}{4}
    & \disp{nan}{4}{nan}{4}
    \\

    &
    $3$-layer $512$-width
    &
    & \disp{5.4365782998502254}{4}{0.08554379646909431}{4}
    & \disp{0.9665873289108277}{4}{0.007167796246648042}{4}
    & \disp{nan}{4}{nan}{4}
    \\
    \hline

    \multirow{3}{*}{WideNorms} &
    $32$-component (each of size $32$)
    &
    & \disp{3.0840566381812096}{4}{0.0666947495805855}{4}
    & \disp{0.7272063374519349}{4}{0.006812639849696139}{4}
    & \disp{nan}{4}{nan}{4}
    \\

    &
    $48$-component (each of size $32$)
    &
    & \disp{3.0437723733484745}{4}{0.13221466253482997}{4}
    & \disp{0.7247223734855652}{4}{0.017345661320886243}{4}
    & \disp{nan}{4}{nan}{4}
    \\

    &
    $128$-component (each of size $32$)
    &
    & \disp{2.9964395333081484}{4}{0.13628229940808578}{4}
    & \disp{0.7172861695289612}{4}{0.016591728852525352}{4}
    & \disp{nan}{4}{nan}{4}
    \\
    \bottomrule
\end{tabular}%
}
\end{adjustbox}
