# Supplementary material for: On the Learning and Learnability of Quasimetrics
Source: arXiv:2206.15478 source file (2022-10-04)
Supplement: Supplementary file 3 [file orth_equi_proof.pdf]

Left

$$\mu \approx n^4 p^4 (1-p)^{10}$$

$$p \gg n^{-1} \\ 1-p \gg n^{-\frac{2}{5}}$$

$$p \gg n^{-\frac{1}{2}} \\ 1-p \gg n^{-\frac{1}{3}}$$

$\Delta^*$

| show        |                      |
|-------------|----------------------|
| $y'$        | $n^3 p^4 (1-p)^9$    |
| $xyw$       | $n^3 p^2 (1-p)^7$    |
| $w$         | $n^3 p^4 (1-p)^8$    |
| $z$         | $n^3 p^4 (1-p)^{10}$ |
| $y' xyw$    | $n^2 p^2 (1-p)^4$    |
| $y' w$      | $n^2 p^4 (1-p)^8$    |
| $y' z$      | $n^2 p^4 (1-p)^9$    |
| $xyw'w$     | $n^2 p^2 (1-p)^4$    |
| $xyw'z$     | $n^2 p (1-p)^6$      |
| $wz$        | $n^2 p^3 (1-p)^9$    |
| $\neg y'$   | $n (1-p)^8$          |
| $\neg xyw'$ | $n p^3 (1-p)^8$      |
| $\neg w$    | $n p (1-p)^3$        |
| $\neg z$    | $n p^2 (1-p)$        |

$\frac{\mu}{\Delta^*}$

|                   |
|-------------------|
| $n (1-p)$         |
| $n p^2 (1-p)^3$   |
| $n (1-p)$         |
| $n$               |
| $n^2 p^2 (1-p)^6$ |
| $n^2 (1-p)^2$     |
| $n^2 (1-p)$       |
| $n^2 p^2 (1-p)^6$ |
| $n^2 p^3 (1-p)^4$ |
| $n^2 p (1-p)$     |
| $n^3 p^4 (1-p)^7$ |
| $n^3 p (1-p)^2$   |
| $n^3 p^3 (1-p)^7$ |
| $n^3 p^2 (1-p)^9$ |

Right

$\Delta^*$

|            |                      |
|------------|----------------------|
| $xy'$      | $n^3 p^3 (1-p)^9$    |
| $yw$       | $n^3 p^3 (1-p)^8$    |
| $z$        | $n^3 p^4 (1-p)^{10}$ |
| $w'$       | $n^3 p^4 (1-p)^9$    |
| $xy' yw$   | $n^2 p^2 (1-p)^4$    |
| $xy' z$    | $n^2 p^2 (1-p)^9$    |
| $xy' w'$   | $n^2 p^3 (1-p)^8$    |
| $yw z$     | $n^2 p^2 (1-p)^7$    |
| $yw w'$    | $n^2 p^3 (1-p)^5$    |
| $z w'$     | $n^2 p^4 (1-p)^9$    |
| $\neg xy'$ | $n p^2 (1-p)^4$      |
| $\neg yw$  | $n p^2 (1-p)^4$      |
| $\neg z$   | $n p^2 (1-p)$        |
| $\neg w'$  | $n p (1-p)$          |

|                   |
|-------------------|
| $n p (1-p)$       |
| $n p (1-p)^2$     |
| $n$               |
| $n (1-p)$         |
| $n^2 p^2 (1-p)^6$ |
| $n^2 p^2 (1-p)$   |
| $n^2 p (1-p)^2$   |
| $n^2 p^2 (1-p)^3$ |
| $n^2 p (1-p)^5$   |
| $n^2 (1-p)$       |
| $n^3 p^2 (1-p)^6$ |
| $n^3 p^2 (1-p)^2$ |
| $n^3 p^2 (1-p)^9$ |
| $n^3 p^4 (1-p)^9$ |

$$p \gg n^{-\frac{3}{4}}$$

$$1-p \gg n^{-\frac{1}{3}}$$

So  $p \gg n^{-2}$   
 $1-p \gg n^{-\frac{1}{3}}$   $\Rightarrow$   $1-o(1)$  prob has both

pair prob.  $\Rightarrow \frac{1}{2} - o(1)$  fail

Iteration

Pick  $\delta$  s.t.  $P(B(n^2, p) \notin [m, m+2\delta]) \rightarrow 0$

$\hookrightarrow$  remove  $\leq 2\delta$  pairs

$P(\text{bad}) \leq 8 \cdot \frac{2\delta}{m}$

$\hookrightarrow$  each remove w.p.  $\leq \frac{2\delta}{m}$

$$\begin{cases} \delta \ll n \sqrt{p(1-p)} \\ p = \frac{m+\delta}{n^2} \end{cases}$$

So need

CASE 1

if  $\frac{m}{n^2} \rightarrow c$  ( $m \sim n^2$ )

$\delta \gg n \sqrt{p(1-p)}$

NOT  $p \ll n^{-\frac{1}{2}}, 1-p \ll n^{-\frac{1}{3}}$

$\delta/m \rightarrow 0$

$\delta = n^{3/2}$

$n \sqrt{p(1-p)}$

$p = \frac{m+\delta}{n^2} \rightarrow c$

$\sim n \frac{(n^2 + n^{3/2}) / n^2}{1 - (n^2 + n^{3/2}) / n^2}$

$\sim n$

so  $\delta \gg n \sqrt{p(1-p)}$

$\frac{\delta}{m} \rightarrow 0$

$p \rightarrow c$  ✓

CASE 2. If  $\frac{m}{n^2} \rightarrow 0$ , but  $\frac{m}{n^2} \gg n^{-\frac{1}{2}}$ ,  $n \gg n^{\frac{3}{2}}$

$$\sqrt{n d p (1-p)} \sim n \sqrt{\frac{m+d}{n^2}} \gg n^{\frac{3}{4}} \quad \frac{d}{m} \rightarrow 0$$

$$\delta = n$$

Then  $\delta \gg \sqrt{n d p (1-p)}$

$$\frac{d}{m} \rightarrow 0$$

$$p = \frac{m+d}{n^2} \gg n^{-\frac{1}{2}} + n^{-1} \sim n^{-\frac{1}{2}}$$

CASE 3. If  $\frac{m}{n^2} \rightarrow 1$ , but  $1 - \frac{m}{n^2} \gg n^{-\frac{1}{3}}$ ,

$$\sqrt{n d p (1-p)} \sim n \sqrt{1 - \frac{m+d}{n^2}} \gg n^{\frac{5}{6}}$$

$$\delta = n^{\frac{11}{6}}$$

$$\frac{d}{m} \rightarrow 0$$

$$1 - p = 1 - \frac{m+d}{n^2} \gg n^{-\frac{1}{3}} - n^{-1} \sim n^{-\frac{1}{3}}$$
