# Supplementary material for: On the Learning and Learnability of Quasimetrics
Source: arXiv:2206.15478 source file (2022-10-04)
Supplement: Supplementary file 4 [file three_nodes.tex]

%auto-ignore
\subsubsection{Additional Results on \Qmet Spaces with Three Elements}

\begin{restatable}[\Qmet Embeddings and PQEs Can Fit Perfectly]{thm}{thmThreeNodesQmetPerfect}
\label{thm:three-nodes-pqe-perfect}
Any \qpmet space $M = (\mathcal{X}, d)$ with $3$ elements admits into an embedding convex combination of $12$ \qparts with distortion $1$ (\ie, perfectly isometric embedding).
For PQEs, there exists a sequence of PQEs uniformly converging a \qmet with \dis $1$, using a $3$-layer ReLU encoder with $6$ hidden width and a $(12l)$-dimensional latent space, where $l$ is the number of latent dimensions needed to parametrize sets in a Poisson process.
\end{restatable}

\paragraph{When $M$  has no infinite distances and is not \emph{\qpmet}, }
this uniform converging PQE sequence essentially implies the existence of a PQE with distortion $1 + \eps$, for any $\eps > 0$, using the above encoder architecture.

\begin{lemma}
\label{lemma:three-nodes-qmet-perfect}
Any \qpmet $d$ on three nodes $\{A, B, C\}$ can be expressed as a convex combination of $12$ \qparts, each of which can be represented as a \emph{total} order. In particular, if $d$ is finite, the convex combination has all finite weights.
\end{lemma}

% \subsubsection{Proof of \Cref{lemma:three-nodes-qmet-perfect}}
\paragraph{Proof strategy.}  In the proof of \Cref{lemma:three-nodes-qmet-perfect} below, we \begin{enumerate}
    \item for finite $d$, formulate the existence of the convex combination as solving a constrained linear programming,
    \item use Farkas' lemma to transform into another program, which has a solution if and only if the original program does not,
    \item show that a solution to the new program would lead to a contradiction using the \qmet properties of $d$, and
    \item extend our results to infinite $d$.
\end{enumerate}

\begin{proof}[Proof of \Cref{lemma:three-nodes-qmet-perfect}]
For simplicity, we represent all \qmets (including \qparts) on $\{A, B, C\}$ as a vector in $[0, \infty]^6$, \eg, \begin{equation}
    \bb{d} \trieq [d(A, B), d(A, C), d(B, C), d(B, A), d(C, A), d(C, B)]\in [0, \infty]^6,
    \label{eq:thm:3node-qmet-solvable-vec-order}
\end{equation}
with $d(A,A)=d(B,B)=d(C,C) = 0$ implicitly.
Furthermore, we will use the subscript to denote the element of the vector, \eg, $\bb{d}_{AB} = d(A, B)$.

\begin{itemize}[leftmargin=20pt]
    \item \myparagraph{Formulation as linear programs for finite $d$ case. }

    For finite $d$, \ie, entries of $\bb{d}$ are all finite, consider the following constrained linear program:
    \begin{equation}
        \bb{P}\T \bb{x} = \bb{d} \quad \text{subject to} \quad \bb{x} \geq 0,
        \label{eq:thm:3node-qmet-solvable-linprog}
    \end{equation}
    where $\bb{P}$ is the $\R^{m \times 6}$ binary valued matrix whose rows are \qparts on $\{A, B, C\}$, and $m$ is the total number of such \qparts.

    It is sufficient to show that \Cref{eq:thm:3node-qmet-solvable-linprog} always has a solution, regardless of $\bb{d}$.

    By Farkas' lemma, we instead show that the following program never has a solution: \begin{equation}
        \bb{P} \bb{y} \geq 0  \quad \text{subject to} \quad  \bb{d}\T\bb{y} < 0.
        \label{eq:thm:3node-qmet-solvable-linprog-farkas-dual}
    \end{equation}

    Let's suppose that $\bb{y}$ solves \Cref{eq:thm:3node-qmet-solvable-linprog-farkas-dual}.

    \item \myparagraph{Two observations about the matrix $\bb{P}$. }

    \begin{enumerate}
        \item
        For any node $X \in \{A, B, C\}$, the followings are two valid \qparts:
        \begin{align}
            p_X^{(1)}(a, b) & = \begin{cases}
                1 & \text{if $a = X$ and $b \neq X$} \\
                0 & \text{otherwise},
            \end{cases} \\
            p_X^{(2)}(a, b) & = \begin{cases}
                1 & \text{if $a \neq X$ and $b = X$} \\
                0 & \text{otherwise},
            \end{cases}
        \end{align}
        where \begin{itemize}
            \item $p_X^{(1)}$ can be understood as the reachability relations of the graph $Y \leftrightarrow Z \rightarrow X$, where the two other nodes can reach each other, \emph{as well as} $X$, but $X$ \emph{can't reach any} other node.
            \item $p_X^{(2)}$ can be understood as the reachability relations of the graph $X \rightarrow Y \leftrightarrow Z$, where the two other nodes can reach each other, \emph{but not} $X$, and $X$ \emph{can reach either} other node,
        \end{itemize}

        By representing these \qparts with the specific ordering in Eqn.~\eqref{eq:thm:3node-qmet-solvable-vec-order}, we know that all $6$ following vectors are valid \qparts and thus rows of $\bb{P}$: \begin{align}
            \bb{p}_A^{(1)} & = [1, 1, 0, 0, 0, 0] \\
            \bb{p}_C^{(2)} & = [0, 1, 1, 0, 0, 0] \\
            \bb{p}_B^{(1)} & = [0, 0, 1, 1, 0, 0] \\
            \bb{p}_A^{(2)} & = [0, 0, 0, 1, 1, 0] \\
            \bb{p}_C^{(1)} & = [0, 0, 0, 0, 1, 1] \\
            \bb{p}_B^{(2)} & = [1, 0, 0, 0, 0, 1].
        \end{align}

        Therefore, we have the following lemma.
        \begin{lemma}\label{lemma:3node-qmet-solvable:2consecutive}
        Any 2 rotationally consecutive entries of $\bb{y}$ must sum to a non-negative value.
        \end{lemma}
        \item
        For any permutation of $\{A, B, C\}$ as $(X, Y, Z)$, the following is a valid \qpart:
        \begin{align}
            p_{XYZ}(a, b) & = \begin{cases}
                0 & \text{if $a = b$} \\
                0 & \text{if $(a, b) \in \{(X, Y), (Y, Z), (X, Z)\}$} \\
                1 & \text{otherwise},
            \end{cases}
        \end{align}
        where $p_{XYZ}$ can be understood as the reachability relations of the graph $X \rightarrow Y \rightarrow Z$.

        Similarly, all $6$ following vectors are valid \qparts and thus rows of $\bb{P}$. \begin{align}
            \bb{p}_{CBA} & = [1, 1, 1, 0, 0, 0] \\
            \bb{p}_{CAB} & = [0, 1, 1, 1, 0, 0] \\
            \bb{p}_{ACB} & = [0, 0, 1, 1, 1, 0] \\
            \bb{p}_{ABC} & = [0, 0, 0, 1, 1, 1] \\
            \bb{p}_{BAC} & = [1, 0, 0, 0, 1, 1] \\
            \bb{p}_{BCA} & = [1, 1, 0, 0, 0, 1],
        \end{align}
        These lead to the following lemma.

        \begin{lemma}\label{lemma:3node-qmet-solvable:3consecutive}
        Any 3 rotationally consecutive entries of $\bb{y}$ must sum to a non-negative value.
        \end{lemma}
    \end{enumerate}

    \item \myparagraph{Proof of certain properties of the solution $\bb{y}$ to \Cref{eq:thm:3node-qmet-solvable-linprog-farkas-dual}.}

    Since $\bb{y}\T \bb{d} < 0$ and $\bb{d} \geq 0$, we necessarily have some negative entry of $\bb{y}$.

    WLOG, let $\bb{y}_{AC} < 0$. By \Cref{lemma:3node-qmet-solvable:2consecutive}, we have \begin{align}
        \bb{y}_{AB} & \geq -\bb{y}_{AC} > 0  \label{eq:thm:3node-qmet-solvable:neg-y-implies-left-neighbor-y-pos}\\
        \bb{y}_{BC} & \geq -\bb{y}_{AC} > 0, \label{eq:thm:3node-qmet-solvable:neg-y-implies-right-neighbor-y-pos}
    \end{align}
    and thus, \begin{align}
        \qquad   & \bb{d}_{AB} - \bb{d}_{AC} + \bb{d}_{BC} \geq 0 \tag {$d$ is a  \qmet} \\
        \implies & \min(\bb{y}_{AB}, \bb{y}_{BC}) \left( \bb{d}_{AB} - \bb{d}_{AC} + \bb{d}_{BC} \right) \geq 0 \notag\\
        \implies & \bb{y}_{AB} \bb{d}_{AB} + \bb{y}_{BC} \bb{d}_{BC} -\min(\bb{y}_{AB}, \bb{y}_{BC}) \bb{d}_{AC} \geq 0 \notag\\
        \implies & \bb{y}_{AB} \bb{d}_{AB} + \bb{y}_{BC} \bb{d}_{BC} + \bb{y}_{AC} \bb{d}_{AC} \geq 0. \label{eq:thm:3node-qmet-solvable:neg-y-implies-3dy-sum-nonneg}
    \end{align}

    % We summarize the above in the following lemma.
    % \begin{lemma}
    % If $\bb{y}_{XZ} < 0$, for some $\{X, Y, Z\} = \{A, B, C\}$, then \begin{enumerate}[topsep=0pt]
    %     \item $\bb{y}_{XY} \geq -\bb{y}_{XZ} > 0$,
    %     \item $\bb{y}_{YZ} \geq -\bb{y}_{XZ} > 0$, and
    %     \item $\bb{y}_{XY} \bb{d}_{XY} + \bb{y}_{YZ} \bb{d}_{YZ} + \bb{y}_{XZ} \bb{d}_{XZ} \geq 0$.
    % \end{enumerate}
    % \end{lemma}

    Since, $\bb{y}\T\bb{d} < 0$, there must be another negative entry of $\bb{y}$. That entry can not be $\bb{y}_{AB}$ or $\bb{y}_{BC}$ by \Cref{eq:thm:3node-qmet-solvable:neg-y-implies-left-neighbor-y-pos,eq:thm:3node-qmet-solvable:neg-y-implies-right-neighbor-y-pos}. It can also not be $\bb{y}_{CA}$; otherwise, by a similar logic we can obtain \begin{equation}
         \bb{y}_{BA} \bb{d}_{BA} + \bb{y}_{CB} \bb{d}_{CB} + \bb{y}_{CA} \bb{d}_{CA} \geq 0,
    \end{equation}
    which together with \Cref{eq:thm:3node-qmet-solvable:neg-y-implies-3dy-sum-nonneg} contradicts with $\bb{y}\T\bb{d} < 0$. Hence, at least one of $\bb{y}_{CB}$ and $\bb{y}_{BA}$ is negative. In fact, we will now show that they both have to be negative.

    WLOG, let $\bb{y}_{CB} < 0$. Since $d$ is a \qmet, we have \begin{equation}
        \bb{d}_{BC} \geq \bb{d}_{AC} - \bb{d}_{AB}. \label{eq:thm:3node-qmet-solvable:vv-not-possible-cond-d}
    \end{equation}
    By \Cref{lemma:3node-qmet-solvable:2consecutive}, we also have \begin{equation}
        \bb{y}_{BC} \geq -\bb{y}_{AC} > 0. \label{eq:thm:3node-qmet-solvable:vv-not-possible-cond-y}
    \end{equation}

    Combining \Cref{eq:thm:3node-qmet-solvable:vv-not-possible-cond-d,eq:thm:3node-qmet-solvable:vv-not-possible-cond-y}, we have \begin{equation}
        \bb{y}_{BC} \bb{d}_{BC}
        \geq -\bb{y}_{AC} \bb{d}_{BC}
        \geq  -\bb{y}_{AC}( \bb{d}_{AC} - \bb{d}_{AB}).
    \end{equation}
    Therefore,
    \begin{equation}
        \bb{y}_{AC} \bb{d}_{AC} + \bb{y}_{BC} \bb{d}_{BC} \geq \bb{y}_{AC}\bb{d}_{AB}.
    \end{equation}
    Similarly, by the same logic, we can obtain
    \begin{equation}
        \bb{y}_{CB} \bb{d}_{CB} + \bb{y}_{CA} \bb{d}_{CA} \geq \bb{y}_{CB}\bb{d}_{AB}.
    \end{equation}
    Combining both, we have \begin{align}
        \bb{y}_{AC} \bb{d}_{AC} + \bb{y}_{BC} \bb{d}_{BC} + \bb{y}_{AB} \bb{d}_{AB} + \bb{y}_{CB} \bb{d}_{CB} + \bb{y}_{CA} \bb{d}_{CA}
        &= (\bb{y}_{AC} + \bb{y}_{AB} + \bb{y}_{CB})\bb{d}_{AB} \notag \\
        & \geq 0,
    \end{align}
    where the last inequality is from \Cref{lemma:3node-qmet-solvable:3consecutive} and the non-negativity of $\bb{d}_{AB}$.

    Therefore, for $\bb{y}\T\bb{d} < 0$, we must have \begin{equation}
        \bb{y}_{BA} \bb{d}_{BA} < 0 \implies \bb{y}_{BA} < 0.
    \end{equation}

    To summarize, we have \begin{align}
        \bb{y}_{AC} & < 0, \\
        \bb{y}_{CB} & < 0, \\
        \bb{y}_{BA} & < 0, \\
        \bb{y}_{CA} & > 0, \\
        \bb{y}_{BC} & > 0, \\
        \bb{y}_{AB} & > 0,
    \end{align}
    where the last three inequalities follows either \Cref{lemma:3node-qmet-solvable:2consecutive} or \Cref{lemma:3node-qmet-solvable:3consecutive}.

    \item \myparagraph{Show by contradiction that $\bb{y}$ can not exist.}

    Finally, we have \begin{align}
        \bb{y}\T\bb{d}
        & = \bb{y}_{BA} \bb{d}_{BA} + \bb{y}_{CA} \bb{d}_{CA} + \bb{y}_{CB} \bb{d}_{CB} + \bb{y}_{AB} \bb{d}_{AB} + \bb{y}_{AC} \bb{d}_{AC} + \bb{y}_{BC} \bb{d}_{BC} \notag \\
        & \geq   \bb{y}_{BA} (\bb{d}_{BC} + \bb{d}_{CA}) + \bb{y}_{CA} \bb{d}_{CA} +
                 \bb{y}_{CB} (\bb{d}_{CA} + \bb{d}_{AB}) + \bb{y}_{AB} \bb{d}_{AB} + \notag \\
        & \qquad \bb{y}_{AC} (\bb{d}_{AB} + \bb{d}_{BC}) + \bb{y}_{BC} \bb{d}_{BC}  \notag\\
        & \tag{$\max(\bb{y}_{AC}, \bb{y}_{CB}, \bb{y}_{BA}) < 0$; $d$ is a quasimetric}  \\
        & =      \bb{d}_{CA} (\bb{y}_{CB} + \bb{y}_{CA} + \bb{y}_{BA}) +
                 \bb{d}_{BC} (\bb{y}_{BA} + \bb{y}_{BC} + \bb{y}_{AC}) + \notag \\
        & \qquad \bb{d}_{AB} (\bb{y}_{AC} + \bb{y}_{AB} + \bb{y}_{CB} ) \notag  \\
        & \geq   \bb{d}_{CA} \cdot 0 +
                 \bb{d}_{BC} \cdot 0 +
                 \bb{d}_{AB} \cdot 0 \notag \\
        & \tag{$\min(\bb{y}_{CA}, \bb{y}_{CB}, \bb{y}_{AB}) > 0$; \Cref{lemma:3node-qmet-solvable:3consecutive}}  \\
        & = 0. \notag
    \end{align}

    Thus, we have a contradiction. So no such $\bb{y}$ exists, and the original problem in \Cref{eq:thm:3node-qmet-solvable-linprog-farkas-dual} would always have a finite solution for any finite \qmet $d$.

    \item \myparagraph{Extension to infinite $d$.}

    For any $d$ with infinite values (\ie, some entry of $\bb{d}$ is $+\infty$), notice that
    \begin{enumerate}
        \item there is a large enough constant $c_d > 0$ \st we can replace all $+\infty$ values in $d$ with $c_d$ and still obtain a valid (now finite) \qmet, denoted as $\tilde{d}$.
        \item the following is also a valid \qmet: \begin{equation}
            d_\mathds{1}(a, b) \trieq \indic{d(a, b) < +\infty}.
        \end{equation}
        In fact, it is a \qpart.
    \end{enumerate}
    Therefore, the original $d$ can be exactly expressed by representing $\tilde{d}$ as a convex combination of \qparts and adding in the extra \qpart $d_\mathds{1}$ with $+\infty$ weight.

    \item \myparagraph{We need only $12$ \qparts that can be represented as \emph{total orders}.}

    By inspecting all \qparts on a $3$-element space, we realize that they can all be represented as convex combinations of these $12$ \qparts shown earlier.
    \begin{align}
        &[1, 1, 0, 0, 0, 0] \\
        &[0, 1, 1, 0, 0, 0] \\
        &[0, 0, 1, 1, 0, 0] \\
        &[0, 0, 0, 1, 1, 0] \\
        &[0, 0, 0, 0, 1, 1] \\
        &[1, 0, 0, 0, 0, 1] \\
        &[1, 1, 1, 0, 0, 0] \\
        &[0, 1, 1, 1, 0, 0] \\
        &[0, 0, 1, 1, 1, 0] \\
        &[0, 0, 0, 1, 1, 1] \\
        &[1, 0, 0, 0, 1, 1] \\
        &[1, 1, 0, 0, 0, 1].
    \end{align}
    Moreover, all such \qparts can be viewed as a \emph{total order} in the sense that for any of these \qpart $d_{01}$, we have $f \colon \{A,B,C\} \rightarrow \R$ such that $d_{01}(X, Y) = 0 \iff f(X) \leq f(Y)$. This can be seen from the alternative view (discussed above) as reachability relations of simple graphs \begin{itemize}
        \item $Y \leftrightarrow Z \rightarrow X$ (\eg, $f(Y) = f(Z) = f(X) - 1$),
        \item $X \rightarrow Y \leftrightarrow Z$ (\eg, $f(Y) = f(Z) = f(X) + 1$), and
        \item $X \rightarrow Y \rightarrow Z$ (\eg, $f(X) + 1 = f(Y) = f(Z) - 1$).
    \end{itemize}
\end{itemize}
This concludes the proof.
\end{proof}

\begin{proof}[Sketch Proof of \Cref{thm:three-nodes-pqe-perfect}]
    Given \Cref{lemma:three-nodes-qmet-perfect}, we know that using $12$ \qparts suffices. For PQEs, following the same arguments as in the proof of \Cref{thm:general-pqpe-low-dis}, we can concentrate the \qpart distributions and/or scale the weights to achieve the desired \dis and uniform convergence with the given architecture. The $12$-dimensional hidden width can also be derived by scrutinizing the proof for \Cref{thm:general-pqe-low-dis} in \Cref{sec:proof-general-pqe-low-dis}.
\end{proof}
