# Supplementary material for: On the Learning and Learnability of Quasimetrics
Source: arXiv:2206.15478 source file (2022-10-04)
Supplement: Supplementary file 5 [file qmet_embedding.tex]

%auto-ignore
%!TEX root = ../../../../main.tex

\subsection{Proofs and Discussions for \Cref{sec:theory-qmet-vioeralization-qmet-emb}: \nameref{sec:theory-qmet-vioeralization-qmet-emb}}

\fixme{talk about an alternative way to look at \vio via mixed \qmet. }

\subsubsection{\Cref{thm:qe-distortion-bounds-vio}: \nameref{thm:qe-distortion-bounds-vio}}

\begin{restatable}[\Qmet Embedding \Dis-Violation Bound]{thm}{thmQEDisBoundsVio}
\label{thm:qe-dis-bounds-vio}
Consider any \qmet space $(\mathcal{X}, d)$ and any training set $S$.
    If $\hat{d}$ is also a \qmet of $\mathcal{X}$, and has \dis $\alpha$ over $S \subset \mathcal{X} \times  \mathcal{X}$, then $\mathcal{V}_{S,d}(\hat{d}) \leq \alpha$.
\end{restatable}

\begin{restatable}[\Qmet Generalization of PQEs]{cor}{corQmetGenPQE}
\label{cor:qmet-vio-pqe}
Consider any \qmet space $(\mathcal{X}, d)$ and any training set $S$ with size $m$. For a PQE with a sufficiently large encoder, \begin{itemize}[topsep=-2pt, itemsep=-2.5pt]
    \item If PQE has $\alpha$ \dis over $S$, its has \vio $\alpha$;
    \item The optimal PQE \wrt \dis has \vio $\bigO(t\log^2 m)$.
\end{itemize}

We have \begin{itemize}[topsep=-2pt, itemsep=-1pt]
    \item For PQEs optimized \wrt \dis over $S$, \begin{itemize}[topsep=-2pt]
        \item If PQE has $\alpha$ \dis over $S$, its has \vio $\alpha$;
        \item The optimal PQE \wrt \dis has \vio $\bigO(t\log^2 m)$.
    \end{itemize}
    \item For PQEs optimized \wrt average \dis over $S \setminus \{(x, x) \colon x \in \mathcal{X}\}$, \begin{itemize}[topsep=-2pt]
        \item If PQE has $\bar{\alpha}$ average \dis over $S$, its has \vio $\bigO(m\alpha)$;
        \item The optimal PQE \wrt \dis has \vio $\bigO(tm\log^2 m)$.
    \end{itemize}
\end{itemize}
\end{restatable}

% \thmQEDistortionBoundsVio*

% \subsubsection{Proof of \Cref{lemma:qe-distortion-bounds-vio}}

\begin{proof}[Proof of \Cref{thm:qe-distortion-bounds-vio}]

Recall the definition of \qmet \vio of predictor $\hat{d}$ trained on $S \subset \mathcal{X} \times  \mathcal{X}$:
 \begin{equation}
    \mathcal{V}_{S,d}(\hat{d}) \trieq \max_{
    \substack{
    (A_1, \dots, A_k) \in \mathcal{X}^{\N+3}\\[1.5pt]
    \exists i, A_i \in S
    }} \frac{d_\mathsf{mix}(A_1, A_k)
    }{d_\mathsf{mix}(A_1, A_2) + d_\mathsf{mix}(A_2, A_3) + \dots + d_\mathsf{mix}(A_{k-1}, A_k)},
\end{equation}
where
\begin{equation}
    d_\mathsf{mix}(a, b) \trieq \begin{cases*}
        d(a, b) & if $(a, b) \in S$ \\
        \hat{d}(a, b) & otherwise.
    \end{cases*} \label{eq:dmix}
\end{equation}

Since \qmet $\hat{d}$ has distortion $\alpha$ over $S$, for any pair $(A_i, A_j) \in S$, \begin{equation}
    0 \leq \frac{1}{\alpha} \hat{d}(A_i, A_j) \leq d(A_i, A_j) \leq \alpha d(A_i, A_j).
\end{equation}

There are five case depending on whether $(A_1, A_k) \in S$ and whether part, all, or none of $\{(A_i, A_{i+1})\}_{i=1,\dots,k-1}$  belong to $S$:
\begin{itemize}
    \item \textbf{Case 1:} $(A_1, A_k) \in S$ and \emph{none} of $\{(A_i, A_{i+1})\}_{i=1,\dots,k-1}$  belong to $S$. We have\begin{align*}
    & \hphantom{ = }    \frac{d_\mathsf{mix}(A_1, A_k)
    }{d_\mathsf{mix}(A_1, A_2) + d_\mathsf{mix}(A_2, A_3) + \dots + d_\mathsf{mix}(A_{k-1}, A_k)} \\
    & = \frac{d(A_1, A_k)}{\hat{d}(A_1, A_2) + \hat{d}(A_2, A_3) + \dots + \hat{d}(A_{k-1}, A_k)}\\
    & \leq \frac{\alpha \cdot \hat{d}(A_1, A_k)}{\hat{d}(A_1, A_2) + \hat{d}(A_2, A_3) + \dots + \hat{d}(A_{k-1}, A_k)} \tag{because $(A_1, A_k) \in S$}\\
    & \leq \alpha.
    \end{align*}

    \item \textbf{Case 2:}  $(A_1, A_k) \notin S$ and \emph{all} of $\{(A_i, A_{i+1})\}_{i=1,\dots,k-1}$  belong to $S$. We have\begin{align*}
    & \hphantom{ = }    \frac{d_\mathsf{mix}(A_1, A_k)
    }{d_\mathsf{mix}(A_1, A_2) + d_\mathsf{mix}(A_2, A_3) + \dots + d_\mathsf{mix}(A_{k-1}, A_k)} \\
    & = \frac{\hat{d}(A_1, A_k)}{d(A_1, A_2) + d(A_2, A_3) + \dots + d(A_{k-1}, A_k)}\\
    & \leq \frac{\hat{d}(A_1, A_k)}{\frac{1}{\alpha}\hat{d}(A_1, A_2) + \frac{1}{\alpha}\hat{d}(A_2, A_3) + \dots + \frac{1}{\alpha}\hat{d}(A_{k-1}, A_k)}\tag{because $\{(A_i, A_{i+1})\}_i \subset S$}\\
    & \leq \alpha  \frac{d(A_1, A_k)}{d(A_1, A_2) + d(A_2, A_3) + \dots + d(A_{k-1}, A_k)}\\
    & \leq \alpha.
    \end{align*}

    \item \textbf{Case 3:}  $(A_1, A_k) \notin S$ and \emph{some but not all} of $\{(A_i, A_{i+1})\}_{i=1,\dots,k-1}$  belong to $S$. WLOG, for notation simplicity, say $k = 3$, $(A_1, A_3) \in S$, $(A_1, A_2) \in S$, and $(A_2, A_3) \notin S$. The argument below holds generally. We have
    \begin{align*}
    & \hphantom{ = }    \frac{d_\mathsf{mix}(A_1, A_k)
    }{d_\mathsf{mix}(A_1, A_2) + d_\mathsf{mix}(A_2, A_3) + \dots + d_\mathsf{mix}(A_{k-1}, A_k)} \\
    & = \frac{d_\mathsf{mix}(A_1, A_3)}{d_\mathsf{mix}(A_1, A_2) + d_\mathsf{mix}(A_2, A_3)} \\
    & = \frac{\hat{d}(A_1, A_3)}{d(A_1, A_2) + \hat{d}(A_2, A_3)} \\
    & \leq \frac{\hat{d}(A_1, A_3)}{\frac{1}{\alpha}\hat{d}(A_1, A_2) + \hat{d}(A_2, A_3)} \tag{because $(A_1, A_2) \in S$} \\
    & \leq \frac{\hat{d}(A_1, A_3)}{\frac{1}{\alpha}\hat{d}(A_1, A_2) + \frac{1}{\alpha}\hat{d}(A_2, A_3)} \\
    & = \alpha \frac{\hat{d}(A_1, A_3)}{\hat{d}(A_1, A_2) + \hat{d}(A_2, A_3)} \\
    & \leq \alpha.
    \end{align*}

    \item \textbf{Case 4:}  $(A_1, A_k) \in S$ and \emph{some but not all} of $\{(A_i, A_{i+1})\}_{i=1,\dots,k-1}$  belong to $S$. Again, WLOG, for notation simplicity, say $k = 3$, $(A_1, A_3) \in S$, $(A_1, A_2) \in S$, $(A_2, A_3) \notin S$, $A_1 \neq A_3$, and $A_1 \neq A_2$. The argument below holds generally. We have
    \begin{align*}
    & \hphantom{ = }    \frac{d_\mathsf{mix}(A_1, A_k)
    }{d_\mathsf{mix}(A_1, A_2) + d_\mathsf{mix}(A_2, A_3) + \dots + d_\mathsf{mix}(A_{k-1}, A_k)} \\
    & = \frac{d_\mathsf{mix}(A_1, A_3)}{d_\mathsf{mix}(A_1, A_2) + d_\mathsf{mix}(A_2, A_3)} \\
    & = \frac{d(A_1, A_3)}{d(A_1, A_2) + \hat{d}(A_2, A_3)}.
    %  \\
    % & \leq \frac{\hat{d}(A_1, A_3)}{\frac{1}{\alpha}\hat{d}(A_1, A_2) + \hat{d}(A_2, A_3)} \tag{because $(A_1, A_2) \in S$} \\
    % & \leq \frac{\hat{d}(A_1, A_3)}{\frac{1}{\alpha}\hat{d}(A_1, A_2) + \frac{1}{\alpha}\hat{d}(A_2, A_3)} \\
    % & = \alpha \frac{\hat{d}(A_1, A_3)}{\hat{d}(A_1, A_2) + \hat{d}(A_2, A_3)} \\
    % & \leq \alpha.
    \end{align*}
    From here, na\"{i}vely proceeding would lead to a $\alpha^2$ bound. However, we can do better by considering the following three cases: \begin{itemize}
        \item \textbf{Case 4a:} If $d(A_1, A_3) \leq \alpha\cdot d(A_1, A_2)$, we have \begin{align*}
            & \hphantom{ = }    \frac{d_\mathsf{mix}(A_1, A_k)
            }{d_\mathsf{mix}(A_1, A_2) + d_\mathsf{mix}(A_2, A_3) + \dots + d_\mathsf{mix}(A_{k-1}, A_k)} \\
            & = \frac{d(A_1, A_3)}{d(A_1, A_2) + \hat{d}(A_2, A_3)} \\
            & \leq \frac{d(A_1, A_3)}{d(A_1, A_2)} \\
            & \leq \alpha.
        \end{align*}

        \item \textbf{Case 4b:} If $d(A_1, A_2) \geq \hat{d}(A_1, A_2)$, we have \begin{align*}
            & \hphantom{ = }    \frac{d_\mathsf{mix}(A_1, A_k)
            }{d_\mathsf{mix}(A_1, A_2) + d_\mathsf{mix}(A_2, A_3) + \dots + d_\mathsf{mix}(A_{k-1}, A_k)} \\
            & = \frac{d(A_1, A_3)}{d(A_1, A_2) + \hat{d}(A_2, A_3)} \\
            & \leq \frac{d(A_1, A_3)}{\hat{d}(A_1, A_2) + \hat{d}(A_2, A_3)} \\
            & \leq \frac{\alpha \cdot \hat{d}(A_1, A_3)}{\hat{d}(A_1, A_2) + \hat{d}(A_2, A_3)} \tag{because $(A_1, A_3) \in S$} \\
            & \leq \alpha.
        \end{align*}

        \item \textbf{Case 4c:} In the remaining case, we have \begin{align}
            d(A_1, A_3) &> \alpha\cdot d(A_1, A_2) \label{eq:distortion-vio-bound-case4c-dist-gt-alpha} \\
            d(A_1, A_2) &< \hat{d}(A_1, A_2).
        \end{align}
        Because $(A_1, A_3) \in S$, $(A_1, A_2) \in S$, and the distortion of $\hat{d}$ over $S$ is $\alpha$, \Cref{eq:distortion-vio-bound-case4c-dist-gt-alpha} implies \begin{equation}
            \hat{d}(A_1, A_3) > \hat{d}(A_1, A_2) \geq 0,\label{eq:distortion-vio-bound-est-dist-gt-ineq}
        \end{equation}
        and, by triangle inequality, \begin{equation}
            \hat{d}(A_2, A_3) \geq \hat{d}(A_1, A_3) - \hat{d}(A_1, A_2) > 0. \label{eq:distortion-vio-bound-est-dist-reverse-tri-ineq-gt-zero}
        \end{equation}
        Denoting $\rho \trieq \frac{d(A_1, A_2)}{\hat{d}(A_1, A_2)} \in (0, 1)$, distortion $\alpha$ over $S$ implies that \begin{equation}
            \frac{d(A_1, A_3)}{\hat{d}(A_1, A_3)} \leq \alpha \rho, \label{eq:distortion-vio-bound-shortcut-pair-ratio-bound}
        \end{equation}
        because $(A_1, A_2) \in S$ and $(A_1, A_3) \in S$.

        Then, we can proceed \begin{align*}
            & \hphantom{ = }    \frac{d_\mathsf{mix}(A_1, A_k)
            }{d_\mathsf{mix}(A_1, A_2) + d_\mathsf{mix}(A_2, A_3) + \dots + d_\mathsf{mix}(A_{k-1}, A_k)} \\
            & = \frac{d(A_1, A_3)}{d(A_1, A_2) + \hat{d}(A_2, A_3)} \\
            & < \frac{d(A_1, A_3)}{d(A_1, A_2) + \hat{d}(A_1, A_3) - \hat{d}(A_1, A_2)} \tag{\Cref{eq:distortion-vio-bound-est-dist-reverse-tri-ineq-gt-zero}} \\
            & = \frac{\hat{d}(A_1, A_3) \frac{d(A_1, A_3)}{\hat{d}(A_1, A_3)}}{\hat{d}(A_1, A_2) \frac{d(A_1, A_2)}{\hat{d}(A_1, A_2)} + \hat{d}(A_1, A_3) - \hat{d}(A_1, A_2)} \\
            & \leq \frac{\hat{d}(A_1, A_3) \cdot \alpha \rho}{\hat{d}(A_1, A_2) \cdot \rho + \hat{d}(A_1, A_3) - \hat{d}(A_1, A_2)} \\
            & \leq \frac{\hat{d}(A_1, A_3) \cdot \alpha \rho}{\hat{d}(A_1, A_2) \cdot (\rho - 1) + \hat{d}(A_1, A_3)} \\
            & < \frac{\hat{d}(A_1, A_3) \cdot \alpha \rho}{\hat{d}(A_1, A_3) \cdot (\rho - 1) + \hat{d}(A_1, A_3)} \tag{\Cref{eq:distortion-vio-bound-est-dist-gt-ineq} and $\rho \in (0, 1)$} \\
            & = \frac{\hat{d}(A_1, A_3) \cdot \alpha \rho}{\hat{d}(A_1, A_3) \cdot \rho} \\
            & = \alpha.
        \end{align*}
    \end{itemize}

    \item \textbf{Case 5:} If $(A_1, A_k) \in S$ and \emph{all} of $\{(A_i, A_{i+1})\}_{i=1,\dots,k-1}$  belong to $S$, we trivially have \begin{align*}
        & \hphantom{ = }    \frac{d_\mathsf{mix}(A_1, A_k)
        }{d_\mathsf{mix}(A_1, A_2) + d_\mathsf{mix}(A_2, A_3) + \dots + d_\mathsf{mix}(A_{k-1}, A_k)} \\
        & = \frac{d(A_1, A_k)}{d(A_1, A_2) + d(A_2, A_3) + \dots + d(A_{k-1}, A_k)}\\
        & \leq 1 \\
        & \leq \alpha.
    \end{align*}

    \item \textbf{Case 6:} If $(A_1, A_k) \notin S$ and \emph{none} of $\{(A_i, A_{i+1})\}_{i=1,\dots,k-1}$  belong to $S$, we also trivially have \begin{align*}
        & \hphantom{ = }    \frac{d_\mathsf{mix}(A_1, A_k)
        }{d_\mathsf{mix}(A_1, A_2) + d_\mathsf{mix}(A_2, A_3) + \dots + d_\mathsf{mix}(A_{k-1}, A_k)} \\
        & = \frac{\hat{d}(A_1, A_k)}{\hat{d}(A_1, A_2) + \hat{d}(A_2, A_3) + \dots + \hat{d}(A_{k-1}, A_k)}\\
        & \leq 1 \\
        & \leq \alpha.
    \end{align*}
\end{itemize}

These conclude the proof.
\end{proof}

\subsubsection{\Cref{cor:qmet-vio-pqe}: \nameref{cor:qmet-vio-pqe}}\label{app:cor:qmet-vio-pqe}

\corQmetGenPQE*

\begin{proof}[Proof of \Cref{cor:qmet-vio-pqe}]
This is a direct consequence of \Cref{thm:general-pqe-low-distortion} and \Cref{thm:qe-distortion-bounds-vio}.
\end{proof}

\paragraph{Other objectives.} \Cref{thm:qe-distortion-bounds-vio} and \Cref{cor:qmet-vio-pqe} provide guarantees for optimizing a \qmet embedding (\eg, a PQE) \wrt distortion. As a result, they also provide certain guarantees for objectives based on distance ratios (\eg, relative error) and log distancves (\eg, MSE on log distances), with possibly weaker bounds. Other objectives, such as MSE on raw distances or discounted distances, focuses on the overall average error, rather than the worst case error. Therefore, to better characterize their behavior, an alternative approach with an average-case analysis might be necessary.
